# Supplementary material for: Practical Conformer: Optimizing size, speed and flops of Conformer for on-Device and cloud ASR
Source: arXiv:2304.00171 source file (2023-03-31)
Supplement: Supplementary file 1 [file appendix.tex]

\section{Appendix}
\label{sec:appendix}

\subsection{Implicit attention computations in Performers}
\label{sec:causal_performer}
Here we summarize implicit attention computations for the bidirectional and unidirectional (causal) attention in Performers \cite{performers}. 

Performers leverage kernel matrix point of view on the attention matrix.
Assume that the attention matrix $\mathbf{A} \in \mathbb{R}^{L \times L}$ is of the form: 
\begin{equation}
\label{kernel_eq}
\mathbf{A}(i,j) = \mathrm{K}(\mathbf{q}_{i}^{\top},\mathbf{k}_{j}^{\top}),
\end{equation}
where $\mathbf{q}_{i}/\mathbf{k}_{j}$ stands for the $i^{th}/j^{th}$ query/key row-vector in the query tensor $\mathbf{Q}$ or key tensor $\mathbf{K}$ respectively. Furthermore, kernel function $\mathrm{K}:\mathbb{R}^{d} \times \mathbb{R}^{d} \rightarrow \mathbb{R}_{+}$ is defined as follows for the (deterministic or randomized) mapping: $\phi: \mathbb{R}^{d} \rightarrow \mathbb{R}_{+}^{r}$ (for some $r >0$):
\begin{equation}
\label{kernel-def}
\mathrm{K}(\mathbf{x}, \mathbf{y}) = \mathbb{E}[\phi(\mathbf{x})^{\top}\phi(\mathbf{y})].
\end{equation}
We call $\phi(\mathbf{u})$ a \textit{feature map} for $\mathbf{u} \in \mathbb{R}^{d}$. 
For $\mathbf{Q}^{\prime},\mathbf{K}^{\prime} \in \mathbb{R}^{L \times r}$ with rows given as $\phi(\mathbf{q}_{i}^{\top})^{\top}$ and $\phi(\mathbf{k}_{i}^{\top})^{\top}$ respectively,
Equation \ref{kernel-def} leads directly to the efficient bidirectional attention mechanism of the form:
\begin{align}
\begin{split}
    \widehat{\mathrm{Att}_\leftrightarrow} (\mathbf{Q}, \mathbf{K}, \mathbf{V}) = \widehat{\mathbf{D}}^{-1} (\mathbf{Q}^{\prime}((\mathbf{K}^{\prime})^{\top} \mathbf{V})), \\ \widehat{\mathbf{D}} = \mathrm{diag} (\mathbf{Q}^{\prime}((\mathbf{K}^{\prime})^{\top} \mathbf{1}_L) ). 
\end{split}    
\end{align} 
Here $\widehat{\mathrm{Att}_\leftrightarrow}$ stands for the approximate attention and brackets indicate the order of computations. It is easy to see that such a mechanism is characterized by space complexity $O(Lr + Ld + rd)$ and time complexity $O(Lrd)$ as opposed to $O(L^{2}+Ld)$ and $O(L^{2}d)$ of the regular attention. 

For the case of the unidirectional (causal) attention, Performers' computations are similar as for the bidirectional case, but this time the goal is to compute $\mathrm{tril}(\mathbf{Q}^{\prime} (\mathbf{K}^{\prime})^\top) \mathbf{C}$ without constructing and storing the $L \times L$-sized matrix $\mathrm{tril}(\mathbf{Q}^{\prime} (\mathbf{K}^{\prime})^\top)$ explicitly, where
$\mathbf{C}~=~\begin{bmatrix} V & \mathbf{1}_L \end{bmatrix} \in \mathbb{R}^{L \times (d + 1)}$. In order to do so, observe that $\forall 1 \leq i \leq L$:
\begin{align} 
\begin{split}
\label{eq:cumsum}
    [\mathrm{tril}(\mathbf{Q}^{\prime} (\mathbf{K}^{\prime})^\top) \mathbf{C}]_i = \mathbf{G}^\mathrm{PS}_{i,:,:} \times \mathbf{Q}^{\prime}_i, \\
    \mathbf{G}^\mathrm{PS}_{i,:,:} = \sum_{j = 1}^i \mathbf{G}_{j,:,:}, \quad \mathbf{G}_{j,:,:} = \mathbf{K}^{\prime}_j \mathbf{C}_j^\top \in \mathbb{R}^{M \times (d + 1)}
\end{split}    
\end{align}
where $\mathbf{G}, \mathbf{G}^\mathrm{PS} \in \mathbb{R}^{L \times M \times (d + 1)}$ are 3d-tensors. Each slice $\mathbf{G}^\mathrm{PS}_{:,l,p}$ is therefore a result of a prefix-sum (or cumulative-sum) operation applied to $\mathbf{G}_{:,l,p}$: $\mathbf{G}^\mathrm{PS}_{i,l,p} = \sum_{j = 1}^i \mathbf{G}_{i,l,p}$. An efficient algorithm to compute the prefix-sum of $L$ elements takes $O(L)$ total steps and $O(\log L)$ time when computed in parallel. 

\subsubsection{RNNAttention-Performers}

At first glance it seems that Equations \ref{kernel_eq} and \ref{kernel-def} severely restrict the class of the attention mechanisms that can be considered. In practice this is not the case and it turns out that even the most popular regular softmax attention is covered by this setting (with the use of softmax kernel and the positive random feature map mechanism introduced in \cite{performers} to effectively approximate softmax kernel for Transformers applications).

It was however observed in \cite{performers} that often one does not need to use softmax kernel in order to get expressive attention mechanism and the other kernel that works particularly well is the so-called $\mathrm{ReLU}$-kernel defined as:
\begin{equation}
\mathrm{K}_{\mathrm{ReLU}}(\mathbf{x},\mathbf{y}) = \mathrm{ReLU}(\mathbf{x})^{\top}\mathrm{ReLU}(\mathbf{y}),     
\end{equation}
where $\mathrm{ReLU}$ is applied elementwise.
The RNNAttention-Performer uses the following modification of the above ReLU-kernel, proposed in \cite{performer-finetuning}:
\begin{equation}
\label{new-relu}
\mathrm{K}_{\mathrm{ReLU++}}(\mathbf{x},\mathbf{y}) = \mathrm{ReLU}(\mathbf{W}\mathbf{x}+\mathbf{b})^{\top}\mathrm{ReLU}(\mathbf{W}\mathbf{y}+\mathbf{b}),     
\end{equation}
for some trainable $\mathbf{W} \in \mathbb{R}^{r^{\prime} \times r}$, $\mathbf{b} \in \mathbb{R}^{r^{\prime}}$ and $r^{\prime} > 0$.
Note that since $\mathbf{x},\mathbf{y}$ correspond to queries and keys that are themselves trainable linear transformations of the inputs to the attention layer, the new kernel is in fact equivalent to:  
\begin{equation}
\label{new-relu}
\mathrm{K}_{\mathrm{shiftedReLU}}(\mathbf{x},\mathbf{y}) = \mathrm{ReLU}(\mathbf{x}+\mathbf{b})^{\top}\mathrm{ReLU}(\mathbf{y}+\mathbf{b}),     
\end{equation}
i.e. the "shifted" version of the ReLU-kernel.

\section{Bidirectional-attention encoder: ablation experiments over different Conformer-Performers}
\label{sec:performers-ablations}

To choose optimal Performer variant, we run ablations over different attention kernels for Performers in the bidirectional encoder setting trained on the $\mathrm{LibriSpeech}$ data. Tested attention kernels $\mathrm{K}:\mathbb{R}^{d} \times \mathbb{R}^{d} \rightarrow \mathbb{R}$ included in particular thoseof the form:  
\begin{equation}
\mathrm{K}_{f}(\mathbf{x},\mathbf{y}) = f(\mathbf{x})^{\top}f(\mathbf{y})    
\end{equation}
for a function $f:\mathbb{R} \rightarrow \mathbb{R}$ applied elementwise to kernel inputs.
We benchmarked the following functions $f$:
\begin{itemize}
\item $f(z) = \mathrm{ReLU}(z)$,
\item $f(z) = \mathrm{SoftPlus}(z)$,
\item $f(z) = \exp(z)$,
\item $f(z) = \mathrm{ELU}(z)$,
\item $f(z) = z^{4}$.
\end{itemize}
All Performer variants were tested in two different settings:
\begin{itemize}
    \item shorter-context: ConformerLGN architecture processing lengths $L \approx 500$
    \item longer-context: ConformerLNS architecture processing lengths $L \approx 800$.
\end{itemize}
In the deterministic kernel feature setting, we found: $f(z) = \mathrm{ReLU}(z)$ and $f(z) = z^{4}$ and $f(z) = \exp(z)$ to be the most efficient functions defining attention kernels (see: Table \ref{tab:perf-abla}). 

\begin{table}[h!]
    \centering
    \caption{Accuracy loss for the Performer-uptrained ConformerLGN.}
    \begin{tabular}{|c|c|c|c|} \hline
    $f(z)$ & $\mathrm{devother}$ & $\mathrm{testother}$ & \# of uptraining steps \\
    & (accuracy loss) & (accuracy loss) & latency (ms)  \\ \hline
    $\exp(z)$ & 0.076\% & 0.095\%  &  31K, 31K  \\ \hline 
    $\mathrm{ReLU}(z)$ & 0.122\% & 0.091\%  & 49K, 31K  \\ \hline 
    $\mathrm{z^{4}}$ & \textbf{-0.012}\% & 0.011\% & 28K, 32K  \\ \hline 
    \end{tabular}
    \label{tab:perf-abla}
\end{table}

\textcolor{red}{TODO: Add more results: plots, speedup numbers, etc.}
